# Supplementary material for: How water wets and self-hydrophilizes nanopatterns of physisorbed hydrocarbons
Source: arXiv:2107.12129 ancillary file (2021-07-26)
Supplement: Supplementary file 1 [file Supplementary_Material_DDiaz.pdf]

## Supplementary Material

### How water wets and self-hydrophilizes nanopatterns of physisorbed hydrocarbons

Diego Díaz<sup>a,h</sup>, Ole Nickel<sup>b</sup>, Hugo Zelada<sup>a</sup>, Rodrigo E. Catalán<sup>a</sup>, María José Retamal<sup>a</sup>, Nicolás Moraga<sup>a</sup>, Marcelo Cisternas<sup>a</sup>, Robert Meißner<sup>b</sup>, PatrickHuber<sup>c,d,e,\*</sup>, Tomas P. Corrales<sup>f,\*</sup>, Ulrich G. Volkmann<sup>a,g,\*</sup>

<sup>a</sup>Instituto de Física, Pontificia Universidad Católica de Chile, Santiago 7820436, Chile

<sup>b</sup>Hamburg University of Technology, Institute of Polymers and Composites, 21073Hamburg, Germany

<sup>c</sup>Hamburg University of Technology, Chair for the Physics of Functional Materials, 21073Hamburg, Germany

<sup>d</sup>Deutsches Elektronen-Synchrotron DESY, Centre for X-Ray and Nano Science CXNS,22603 Hamburg, Germany

<sup>e</sup>University of Hamburg, Centre for Hybrid Nanostructures CHyN, 22607 Hamburg,Germany

<sup>f</sup>Departamento de Física, Universidad Técnica Federico Santa María, Valparaiso 2390123, Chile

<sup>g</sup>Centro de Investigación en Nanotecnología y Materiales Avanzados (CIEN-UC), Pontificia Universidad Católica de Chile, Santiago 7820436, Chile

<sup>h</sup>Max Planck Institute for Polymer Research, Ackermannweg 10, D-55128, Mainz, Germany

\* Corresponding authors: [patrick.huber@tuhh.de](mailto:patrick.huber@tuhh.de), [tomas.corrales@usm.cl](mailto:tomas.corrales@usm.cl), [volkmann@fis.puc.cl](mailto:volkmann@fis.puc.cl)

## Electron microscopy

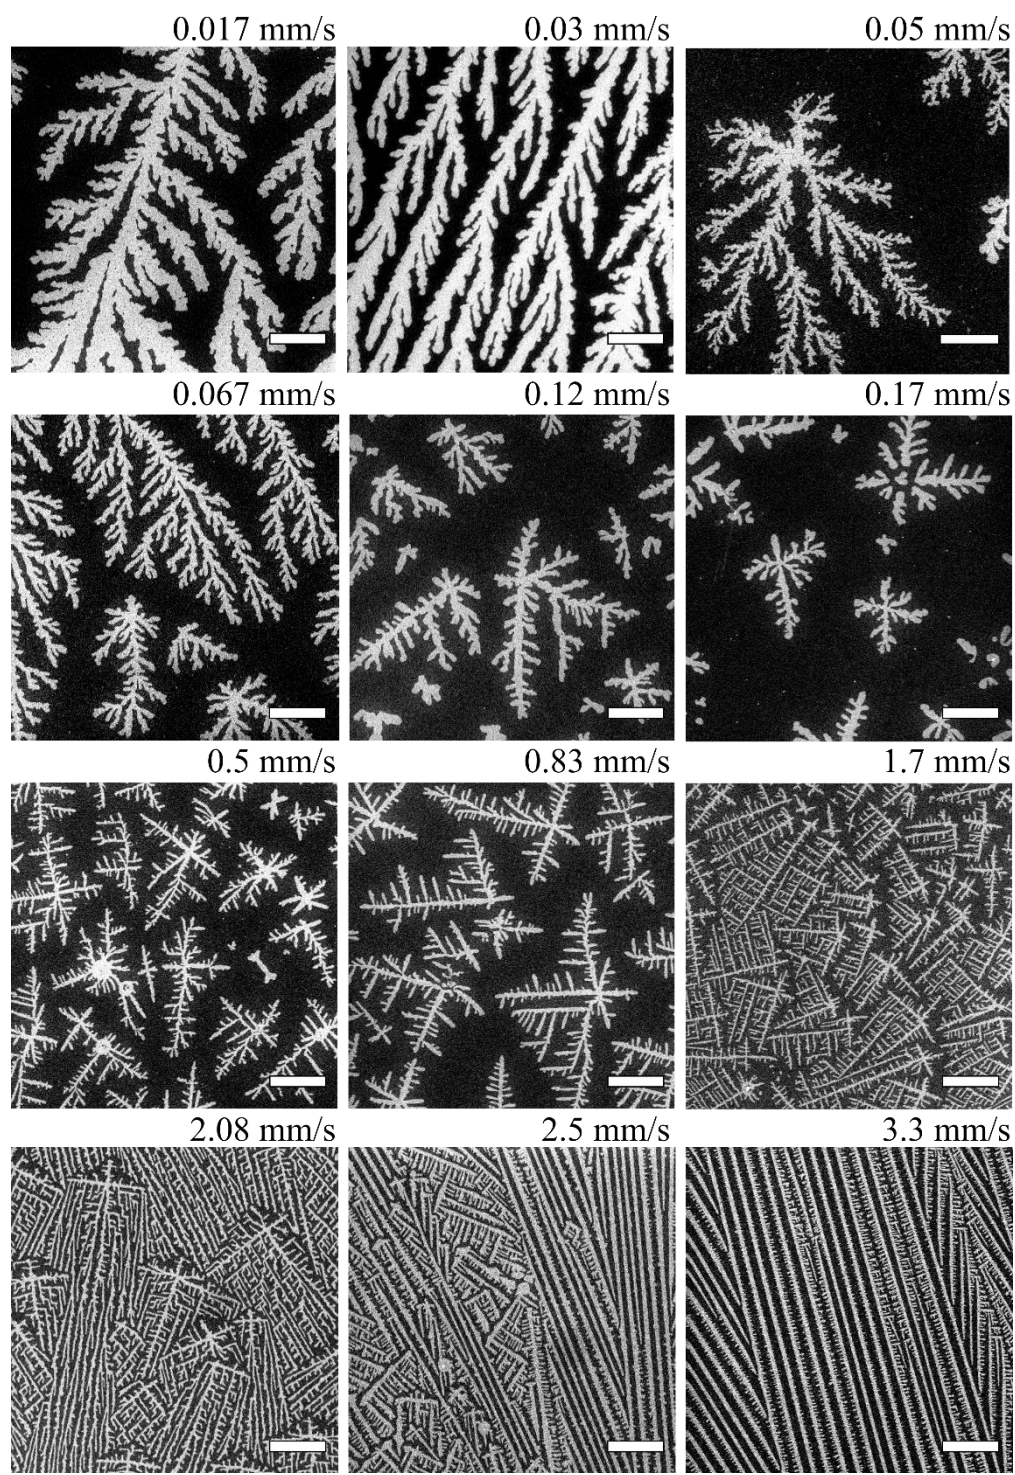

Figure S1: Representative electron micrographs of all pulling velocities used to prepare samples. The white scale bar represents 10  $\mu\text{m}$ .

### Step Height of nanopatterns measured by AFM

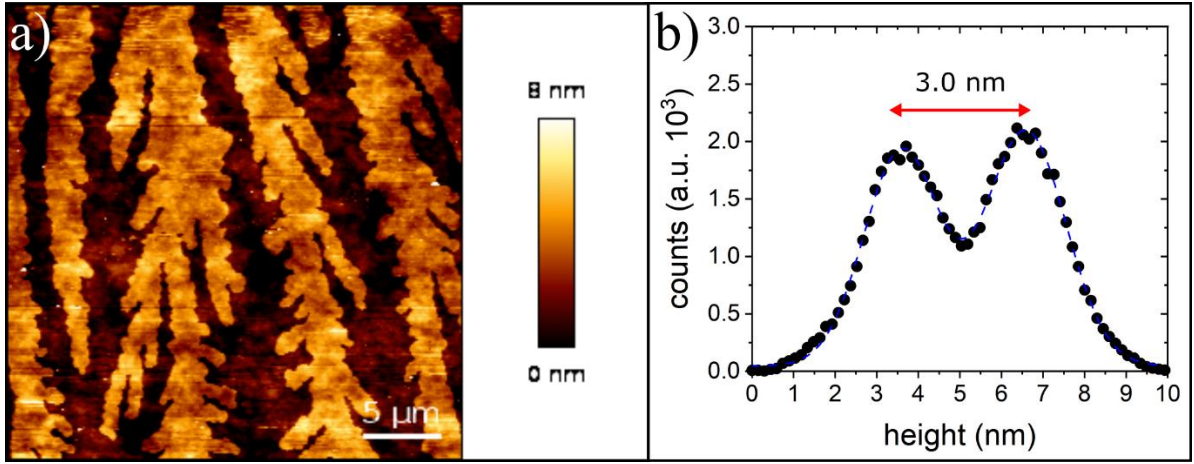

Figure S2: a) AFM image of a sample in dry conditions right after preparation at the lowest pulling velocity (0.017 mm/s). b) Height histogram of the AFM image showing an average height of 3 nm.

### Average film height of the nanopatterns

The average film thickness is defined by:

$$\langle h \rangle = \frac{1}{N} \sum_i^N h_i$$

where  $h_i$  is the height at a position  $i$  over the surface and  $N$  is the number positions into which the entire surface is divided, i.e. a grid of positions. The number of grid positions over the entire surface  $N$  is such that the area covered by each individual position is equal to the area occupied by a single perpendicular molecule of C32:  $\delta A$ . This means that the total area of the sample is  $N\delta A$ . Given that the film consists of only a single perpendicular molecule of length  $l$  over the complete surface, then:

$$h_i = l \cdot g_i$$

Here  $g_i$  is a piecewise function valued 1 when there is a molecule at position  $i$ , and 0 if there is no perpendicular molecular in position  $i$ .

$$g_i = \begin{cases} 1, & \text{molecule in position } i \\ 0, & \text{No molecule in position } i \end{cases}$$

Therefore:

$$\langle h \rangle = \frac{l}{N} \sum_i^N g_i$$

By introducing the area of a single molecule ( $\delta A$ ):

$$\langle h \rangle = \frac{l}{N\delta A} \sum_i^N g_i \delta A$$

Here we can see that the total area of the sample is  $A_{total} = N\delta A$  and the area covered by our nanopattern is actually  $A_{C32} = \sum_i^N g_i \delta A$ . Therefore:

$$\langle h \rangle = \frac{l}{A_{total}} A_{C32}$$

We can see from here that fraction covered by our nanopattern ( $f_1$ ), measured from SEM micrographs, is in fact the term  $A_{C32}/A_{total}$ , and thus:

$$\langle h \rangle = l \cdot f_1 \quad (\text{eq. 1})$$

Using our measured coverage percentage ( $100 \cdot f_1$ ), obtained from SEM, we can calculate the average film thickness of all our samples, considering the molecular length  $l = 4.3 \text{ nm}$ .

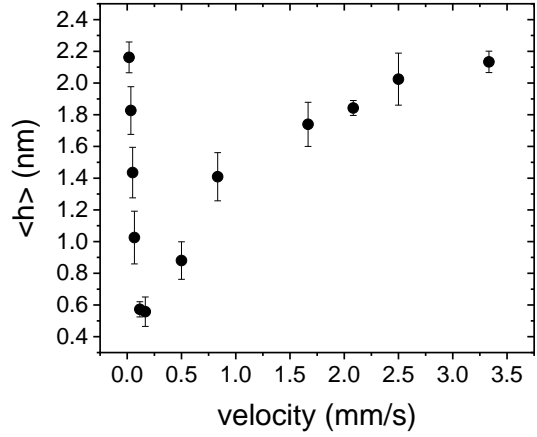

Figure S3: Average film thickness as a function of pulling velocity.

### Surface roughness of the nanopatterns

The roughness of the sample can be obtained by the definition of RMS roughness:

$$R_Q = \sqrt{\frac{1}{N} \sum_i^N (h_i - \langle h \rangle)^2} = \sqrt{\langle h^2 \rangle - \langle h \rangle^2}$$

By using the equation for average height (eq.1):

$$R_Q = \sqrt{\langle h^2 \rangle - l^2 f_1^2}$$

The average square height at position  $i$  can be rewritten yielding:

$$R_Q = \sqrt{\frac{1}{N} \sum_i^N h_i^2 - l^2 f_1^2}$$

By using the previous definition of  $h_i = l \cdot g_i$ :

$$R_Q = \sqrt{\frac{1}{N} \sum_i^N l^2 g_i^2 - l^2 f_1^2}$$

Given the definition of  $g_i$ , it can only take values of 0 or 1 depending on whether a molecule is present in the position or not. Because of this definition, the function  $g_i^2 = g_i$ , and therefore:

$$R_Q = \sqrt{\frac{1}{N} \sum_i^N l^2 g_i - l^2 f_1^2}$$

By introducing the area occupied by a single perpendicular molecule  $\delta A$ :

$$R_Q = \sqrt{\frac{1}{N\delta A} \sum_i^N g_i \delta A - l^2 f_1^2}$$

Finally, we note that the total area is  $A_{total} = N\delta A$  and the area covered by the nanopattern  $A_{C32} = \sum_i^N g_i \delta A$ , hence:

$$R_Q = \sqrt{l^2 f_1 - l^2 f_1^2}$$

Factorizing this expression, we obtain Equation 2:

$$R_q = l\sqrt{f_1 \cdot (1 - f_1)} \quad (\text{eq. 2})$$

Which is consistent with the system, i.e., if the surface is totally filled with molecules ( $f_1 = 1$ ) the surface roughness is 0, while if there are no molecules ( $f_1 = 0$ ), the roughness is also zero. Using this equation, we can obtain a plot for surface roughness versus velocity:

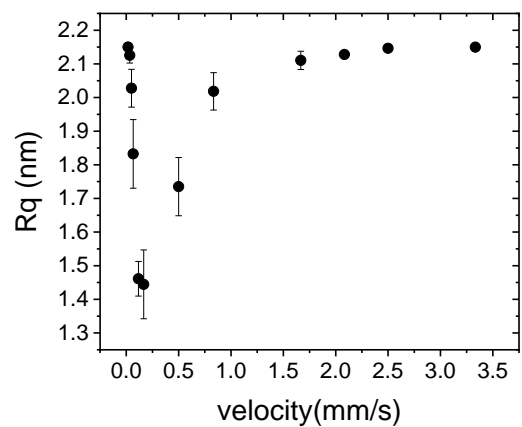

Figure S4: Roughness versus preparation velocity.

From Figure S4, we see that the surface roughness varies  $\sim 0.6$  nm between all samples. Most samples have roughness between 2.0 and 2.1 nm. Using this calculated roughness, we can plot the corresponding contact angle versus roughness:

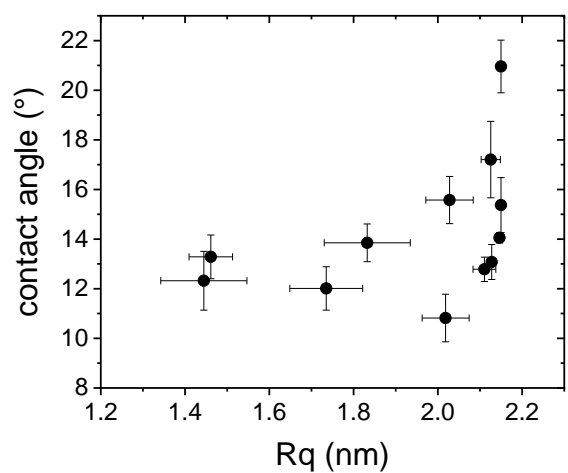

Figure S5: Contact angle versus the calculated roughness.

### Surface Roughness from AFM measurements in dry conditions

From the AFM measurements, we measured the roughness ( $R_q$ ) of samples prepared at dip-coating velocities: 0.033, 1.7 and 3.3 mm/s in dry conditions and under water. The measured roughness values were 2.3 nm, 1.8 nm and 1.8 nm, respectively, for samples in dry conditions, which is in good agreement with the results shown in Figures S2.

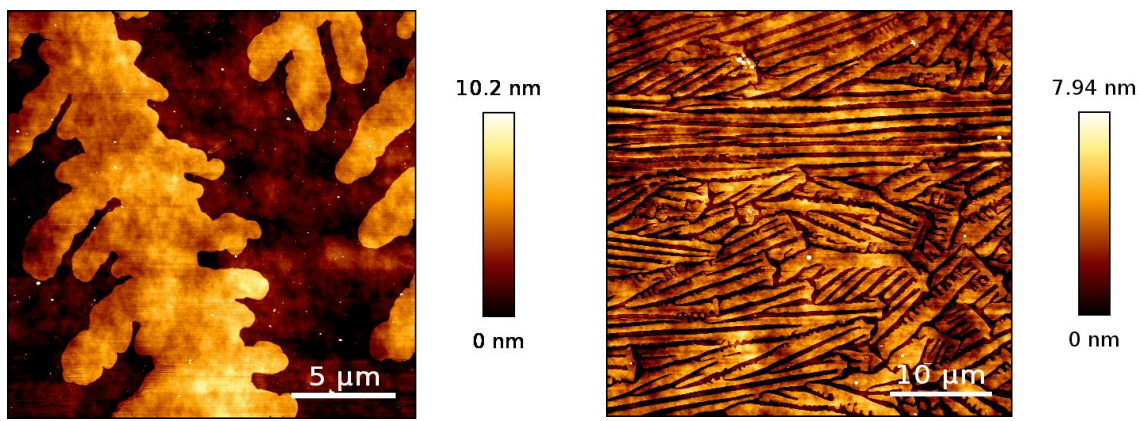

Figure S6. AFM in air of sample prepared at dip-coating velocity 0.033 mm/s (left image) and 1.7 mm/s (right image). The surface roughness is 2.3 nm and 1.8 nm, respectively.

### Surface Roughness from AFM measurements in water

After the AFM measurements in dry conditions (air), the same samples were immersed in water to study stability of the nanopatterns and the change in roughness. The sample prepared at 0.033 mm/s and 1.7 mm/s have an  $R_q$  roughnesses of 4.4 nm and 7.4 nm, respectively. The Sample prepared at 3.3 mm/s, which is shown in the main text Figure 5b has a roughness of 11.6 nm.

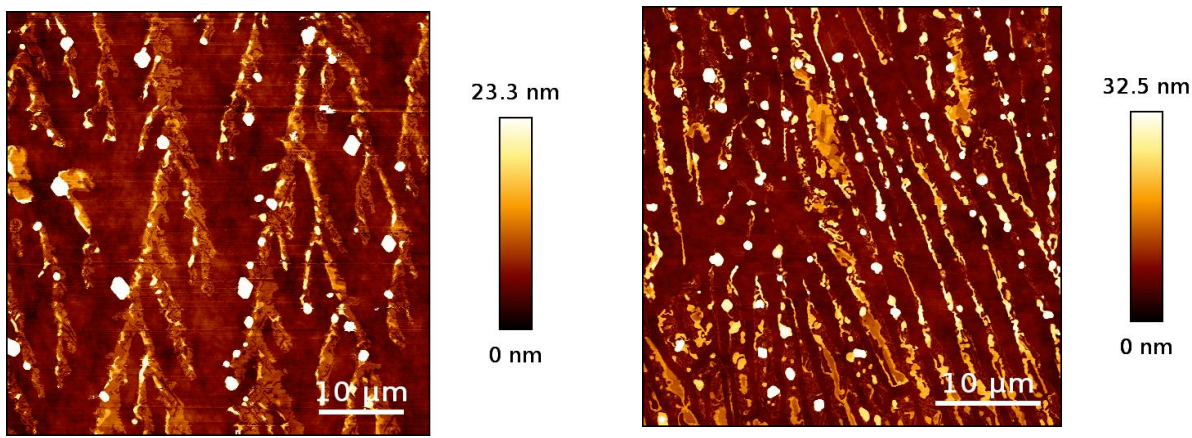

Figure S7. Left: Sample prepared at dip-coating velocity 0.033 mm/s immersed in liquid. Right: Sample prepared at dip-coating velocity at 1.7 mm/s immersed in liquid. The roughness of both samples are 4.4 nm and 7.4 nm, respectively.

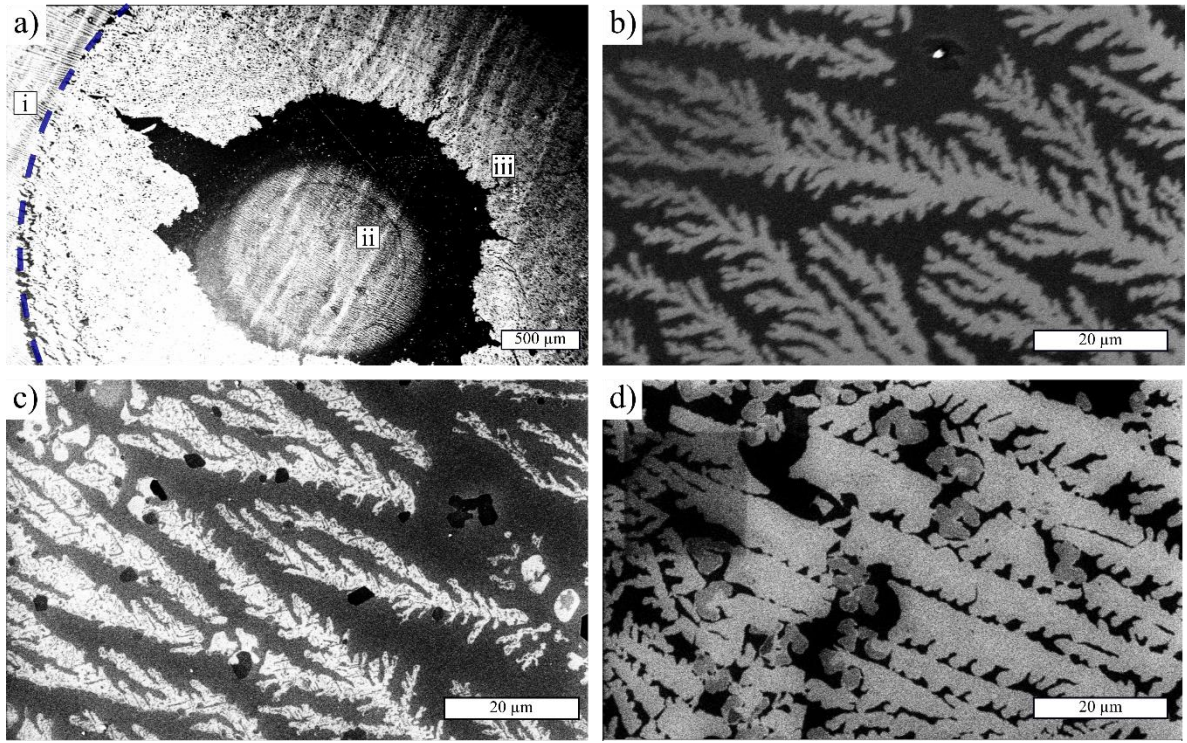

Figure S8: a) Low magnification of the area where the droplet is placed after its complete evaporation. The blue dashed line indicates the limit of the droplet. Here we distinguish three regions: i, ii and iii. b) SEM image of region i, which is unaffected by the liquid droplet. c) Region ii that lies in the center of the liquid droplet and is restructured under the effect of the liquid. d) Region iii is an intermediate region that we believe is being restructured by the moving contact line and does not resemble the original nanopattern.
